# Supplementary material for: Auto-Tables: Synthesizing Multi-Step Transformations to Relationalize Tables without Using Examples
Source: arXiv:2307.14565 source file (2023-08-09)
Supplement: Supplementary file 1 [file apx-additional-operators.tex]

\section{Additional Operators}
\label{apx:additional-op}

\textbf{Explode.} \code{Explode}~\cite{op-explode} is an operator that converts columns with composite values (which violates the First Normal Form~\cite{codd1990relational}), into atomic values. This is shown in Figure~\ref{fig:op-explode} -- notice that the ``\code{Protein IDs}'' column contain multiple values separated by ``;'', making it non-relational and hard to query (e.g., filter and aggregate). An \code{explode} would convert each atomic value into a separate row, making the resulting table more amenable to analysis.

\begin{figure}[h]
    \centering
    \includegraphics[width=0.8\columnwidth]{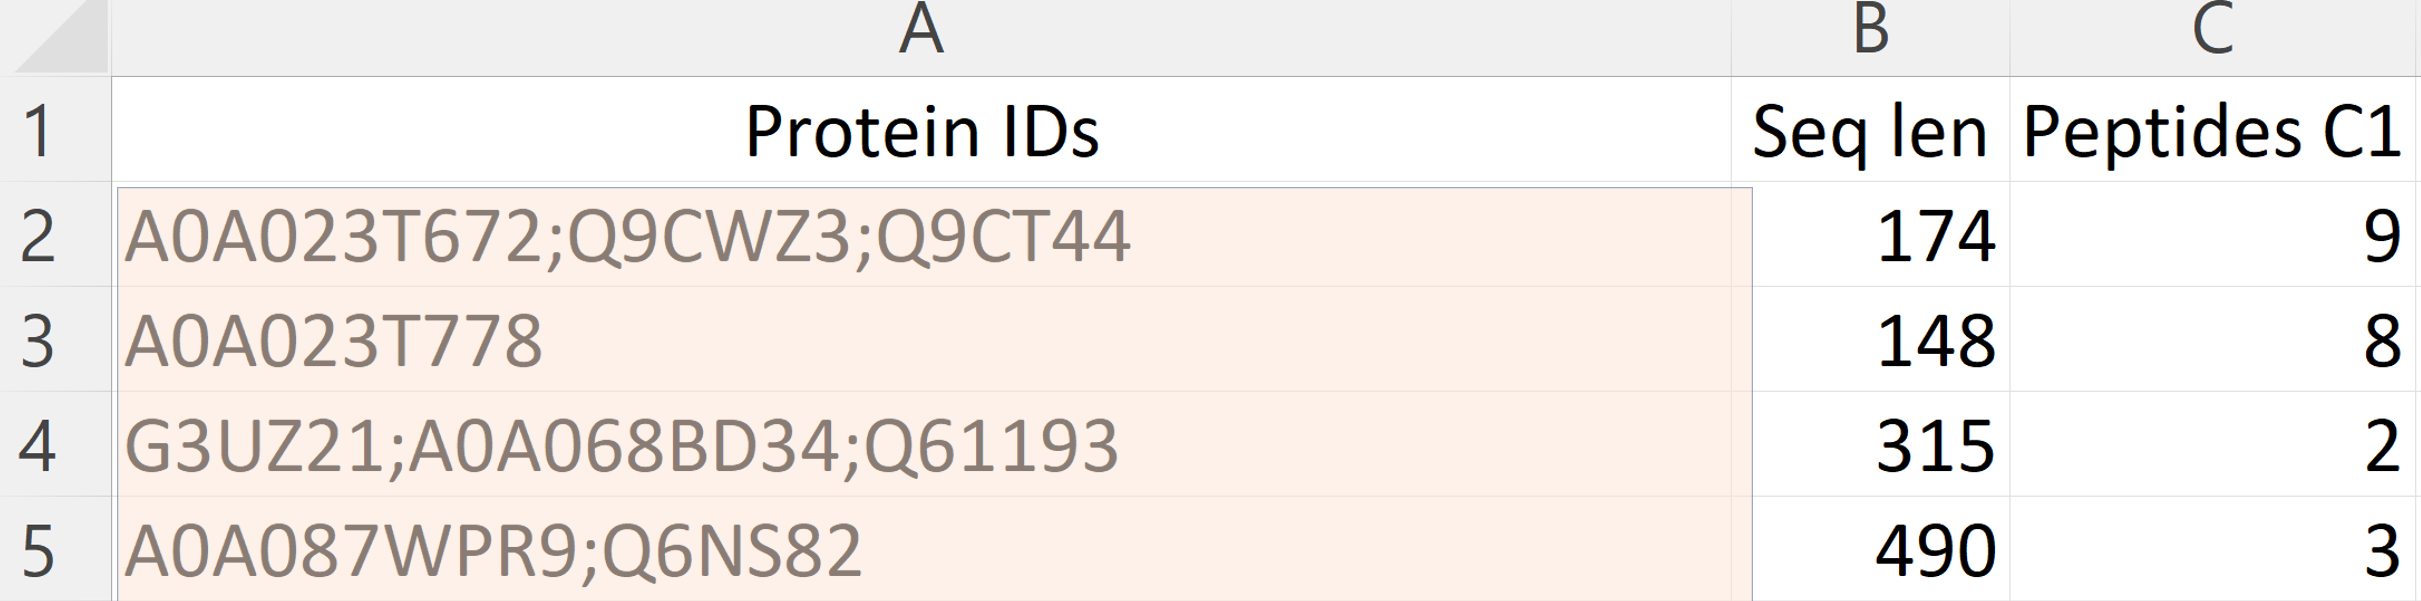}
    %\vspace{-8mm}
    \caption{Example for explode.}
    \label{fig:op-explode}
%\vspace{-5mm}
\end{figure}

\underline{Parameters.} Like shown in Table~\ref{tab:dsl}, the \code{explode} operator has 2 parameters, a ``\code{column\_idx}'' parameter to specify which column to operate on (in this case ``\code{Protein IDs}''), and a ``\code{delim}'' parameter that specifies how composite cells can be broken into atomic values (in this case \code{delim}=``;'').

\textbf{Ffill.} \code{ffill}~\cite{op-ffill} is an operator that fills values into structurally empty cells in tables. Unlike empty cells that may occur randomly inside tables,  structurally empty cells  are often organized hierarchically for visual browsing, which are the key visual signals for our algorithms to detect.

\underline{Parameters.} Like operators such as \code{stack}, \code{ffill} requires two parameters, start\_idx and end\_idx, in order to identify columns for which \code{ffill} needs to be performed.

\textbf{Subtitle.} \code{subtitle} is an operator transforms tables that embed sub-title information, which are mixed together with data-rows, but with visual clues, such as being empty for all cells in the same row, to the right of the sub-title cell.

\underline{Parameters.} \code{Subtitle} has two parameters, column\_idx that identifies the column that contains sub-title information, and row\_filter that filters to rows that actually contain sub-titles.

\textbf{None.} \code{None} is special no-op operator, to indicate that an input table is already relational, for which no additional transformation is needed.

\underline{Parameters.} \code{None} requires no parameters, as one can expect.
